# Supplementary material for: Networks of Pendula with Diffusive Interactions
Source: arXiv:2408.02352 source file (2024-08-05)
Supplement: Supplementary file 1 [file relative.tex]

\section{Relative coordinates}\label{app:relative}

We introduce here a new coordinate system that we call \emph{relative coordinates} \rb{cite the other papaers that use these coordinates \cite{henderson1991geometry}},
\begin{align*}
    q_s &:= q_1 - q_2 \\
    p_s &:= p_1 - p_2 \\
    q_a &:= q_1 + q_2 \\
    p_a &:= p_1 + p_2 .\\
\end{align*}
%The domain of bounded motion then becomes $[-2\pi,2\pi]^2 \times \mathbb{R}^2 \simeq \mathbb{T}^2 \times \mathbb{R}^2$. 
We give two interpretations of such coordinates: the first is related to synchrony and anti-synchrony, in fact if $q_s=p_s=0$ the system is in synchrony and if $q_a=p_a=0$ then the system is in anti-synchrony; the second is in terms of center of mass/momentum and relative distance/momentum, indeed $q_a$ and $p_a$ are the coordinates of the center of mass and momentum, while $q_s$ and $p_s$ are the relative position and momentum.

The Hamiltonian in relative coordinates reads
\begin{equation}
    H= \frac{p_s^2 + p_a^2}{2} - 4 \cos{\frac{q_a}{2}} \cos{\frac{q_s}{2}} + 2 \kappa G(q_s,p_s) ,
\end{equation}
and the associated vector field is
\begin{equation}\label{eq:relative_coordinates_system}
    \begin{aligned}
       \dot{q}_s &= p_s + 2 \kappa G_{01}(q_s,p_s) \\
       \dot{q}_a &= p_a \\
       \dot{p}_s &= - 2 \left( \cos{\frac{q_a}{2}} \sin{\frac{q_s}{2}}  + \kappa G_{10}(q_s,p_s) \right)\\
       \dot{p}_a &= - 2 \cos{\frac{q_s}{2}} \sin{\frac{q_a}{2}} .
    \end{aligned}
\end{equation}

We look once again at synchrony and anti-synchrony but in the new coordinates. Synchrony now is given by setting $q_s=p_s=0$,
\begin{equation}
    \begin{aligned}
       \dot{q}_s &= 0 \\
       \dot{q}_a &= p_a \\
       \dot{p}_s &= 0 \\
       \dot{p}_a &= - 2 \sin{\frac{q_a}{2}} ,
    \end{aligned}
\end{equation}
which results in a equilibrium for the $(q_s,p_s)$ coordinates, while $(q_a,p_a)$ follows the evolution of a simple pendulum. Similarly we can look at anti-synchrony by setting $q_a=p_a=0$,
\begin{equation}\label{eq:antisynchrony_relative}
    \begin{aligned}
       \dot{q}_s &= p_s + 2 \kappa G_{01}(q_s,p_s) \\
       \dot{q}_a &= 0 \\
       \dot{p}_s &= - 2 \left( \sin{\frac{q_s}{2}}  + \kappa G_{10}(q_s,p_s) \right)\\
       \dot{p}_a &= 0 ,
    \end{aligned}
\end{equation}
where we have an equilibrium for $(q_a,p_a)$ and the the coordinates $(q_s,p_s)$ evolves like a perturbed pendulum. Despite the different coordinates the description of the invariant spaces remains quite similar to the standard coordinates case. The new coordinate system brings the advantage of having a simpler relation for the invariance, i.e., now a couple of coordinates is static. Moreover, we can give a physical interpretation of the dynamics in the invariant spaces. In the case of synchrony the two `particles' are overlapping for all times, the only evolving quantity is the center of mass/momentum. In other words, when there is synchrony the system is indistinguishable from a single simple pendulum. In the case of anti-synchrony the only evolving quantities are relative position/momentum, which means that the center of mass/momentum is fixed to the initial conditions for all times.
